# Supplementary material for: Trimmed Conformal Prediction for High-Dimensional Models
Source: arXiv:1611.09933 source file (2016-11-29)
Supplement: Supplementary file 1 [file supplement.tex]

\section{Affine constraints and Related computations}
The constraints for sighed support of lasso fit is given in \citet{Lee2016}: the condition is on $\bY$ such that
\begin{equation*}
    A\cdot \bY_y \leq b
\end{equation*}
where $A=A_{M,s}=\begin{bmatrix}A_0(M,s)\\A_1(M,s)\end{bmatrix}$ and $b=b_{M,s}=\begin{bmatrix}b_0(M,s)\\b_1(M,s)\end{bmatrix}$ 
\begin{align*}
    A_0(M,s)&=\frac{1}{\lambda}\begin{pmatrix}X_{-M}^\top(I-P_M)\\-X_{-M}^\top(I-P_M)\end{pmatrix}\\
    b_0(M,s)&=\begin{pmatrix}
    1 - X_{-M}^\top (X_M^\top)^+ s\\1 + X_{-M}^\top (X_M^\top)^+ s
    \end{pmatrix}\\
    A_1(M,s) &= -diag(s)(X_M^\top X_M)^{-1}X_M^\top\\
    b_1(M,s) &= -\lambda diag(s)(X_M^\top X_M)^{-1} s
\end{align*}
where $P_M=X_M(X_M^\top X_M)^{-1}X_M^\top$, and $X_M^+=(X_M^\top X_M)^{-1}X_M^\top$.

Here in the conformal prediction setting, the first $n$ element in $\bY_y$ is given. So the constraints are in the form
\begin{align*}
    A_{i,n+1}\cdot y &<b_i - [A_{i,1},\ldots, A_{i,n}]\cdot [Y_1,\ldots,Y_n]^\top
\end{align*}
for $1\leq i\leq 2p-|M|$. 
The range $[c_{M,s}, d_{M,s}]$ is solved by 
\begin{align*}
    c_{M,s}&= \max_{i|A_{i,n+1}<0}\left\{\frac{b_i- [A_{i,1},\ldots, A_{i,n}]\cdot [Y_1,\ldots,Y_n]^\top}{A_{i,n+1}}\right\}\\
    d_{M,s}&= \min_{i|A_{i,n+1}>0}\left\{\frac{b_i- [A_{i,1},\ldots, A_{i,n}]\cdot [Y_1,\ldots,Y_n]^\top}{A_{i,n+1}}\right\}
\end{align*}

\section{Least square fit for lasso}
Denote $\bY=[\bY_1,\ldots,\bY_n]^\top$, $\tilde{\bX}=[\bX_1^\top,\ldots,\bX_{n+1}^\top]^\top$. 
For trial $y\in [c_{M,s},d_{M,s}]$, that shares the same signed support, the residues can be computed by
\begin{align*}
    |\hat{r}_{\textnormal{lasso}}(y)|
    &= |\tilde{\bX}((\tilde{\bX}_{M}^{+})_{1:n}\bY-\lambda (\tilde{\bX}_{M}^\top \tilde{\bX}_{M})^{-1}s)\\
    &\quad\quad\quad-[\bY^\top,0]^\top+\tilde{\bX}(\tilde{\bX}_{M}^+)_{n+1}y-[\vec{0},y]^\top|\\
    &= |\mathbf{p}-\mathbf{q}y|
\end{align*}
where $\mathbf{p}$ and $\mathbf{q}$ only depends on $\tilde{X}$ and $\bY$ but not $y$. For conformal prediction, we only need to know the residues (and no need for fitted model). Thus we can use the same $\mathbf{p}$ and $\mathbf{q}$ for all the values of $y\in [c_{M,s}, d_{M,s}]$, and do not need to fit $\hat{\beta}_y$, thus avoiding a lot of matrix computation. 

\section{Algorithm for trimming and prediction steps}
The general algorithm is as follows:
\begin{algorithm}
    \caption{TCP}
    \label{algo:trim&pred}
    \SetKwInOut{Input}{Input}
    \SetKwInOut{Output}{Output}

    \underline{function Conformal Prediction with Trimming}\;
    \Input{$X\in\R^{n\times p}$: $n$ sample and $p$ features.\\
    $Y\in\R^{n}$ response variable.\\
    $X_{n+1}\in\R^{1\times p}$ a new sample point.\\
    $\alpha\in(0,1)$ miscoverage rate.\\
    $\atrim$ target trimming miscoverage rate. \\
    $\mathcal{A}_{\textnormal{fast}}$ a fast regression algorithm. \\
    $\mathcal{A}_{\textnormal{slow}}$ a slow regression algorithm. \\
    }
    \Output{$y_{conf}$ conformal prediction interval}
    \tcc{Trimming step}
    $(\rf)_y\gets$ residues of fitting $\mathcal{A}_{\textnormal{fast}}$\;
    $\Ytrim = \Big\{y : \text{Rank$(|((\rf)_y)_{n+1}|)$}>\lceil(n+1)(1-\atrim)\rceil\Big\}$\;
    \tcc{Prediction Step:}
    $(\rs)_y\gets$ residues of fitting $\mathcal{A}_{\textnormal{slow}}$\;
    $\Ypred = \Big\{y : \text{Rank$(|((\rs)_y)_{n+1}|)$}>\lceil(n+1)(1-\alpha+\atrim)\rceil\Big\}$\;
\end{algorithm}

The specific algorithm for $\mathcal{A}_{\textnormal{fast}}=\textnormal{Ridge regression}$ and $\mathcal{A}_{\textnormal{slow}}=\textnormal{lasso}$ is

\begin{algorithm}
    \caption{Lasso-TCP with Ridge Trimming}
    \label{algo:trim&pred}
    \SetKwInOut{Input}{Input}
    \SetKwInOut{Output}{Output}

    \underline{function Lasso-TCP with Ridge Trimming}\;
    \Input{$X\in\R^{n\times p}$: $n$ sample and $p$ features.\\
    $Y\in\R^{n}$ response variable.\\
    $X_{n+1}\in\R^{1\times p}$ a new sample point.\\
    $\alpha\in(0,1)$ miscoverage rate.\\
    $\atrim = \frac{1}{n+1}$ trimming miscoverage rate. \\
    $\rho$ ridge regression penalty.\\
    $\lambda$ lasso penalty.\\
    $y_{trial}$ a trial set of possible $y$ values at $X_{n+1}$.\\
    }
    \Output{$y_{conf}$ conformal prediction interval}
    
    \tcc{Trimming step}
    $\tilde{\bX}\in\R^{(n+1)\times p}=[\bX^\top, X_{n+1}^\top]^\top$\; 
    $\mathbf{u} = \tilde{\bX}(\tilde{\bX}^\top \tilde{\bX} + \rho \mathbf{I}_p)\tilde{\bX}^\top \begin{bmatrix}
    \bY\\ 0\end{bmatrix}- \begin{bmatrix}
    \bY\\ 0\end{bmatrix}$\;
    $\mathbf{v} = \left(\tilde{\bX}(\tilde{\bX}^\top \tilde{\bX} + \rho \mathbf{I}_p)\tilde{\bX}^\top\right)_{n+1}- \begin{bmatrix}
    \vec{0}\\  1\end{bmatrix}$\;
    $(c_i,d_i)_{1\leq i\leq n}\gets \left(\min,\max \right)\textnormal{of} \left(\frac{\mathbf{u}_{n+1}-\mathbf{u}_i}{\mathbf{v}_i - \mathbf{v}_{n+1}}, \frac{-\mathbf{u}_{n+1}-\mathbf{u}_i}{\mathbf{v}_i + \mathbf{v}_{n+1}}\right)$\;
    $\Ytrim \gets [\min(c_i),\max{d_i}]$\;
    \tcc{Prediction Step:}
    
    \For{$y\in \Ytrim$}{
    $\tilde{Y}_y\gets [\bY^\top,y]^\top$\;
    \If{$y\in(c_{M,s},d_{M,s})$}{
        \tcc{Full lasso fit}
        $V\gets$ set of features that violates $A\tilde{Y}_y<b$\;
        \If{$|V|=1$}{$(M,s,A,b)\gets $ signed support $\&$ affine\;
        $\hat{\beta}_y \gets X_{M}^+\tilde{Y}-\lambda (X_{M}^\top X_{M})^{-1}s$\;}
        \Else{$\hat{\beta}_y \gets lasso_\lambda(\tilde{X},\tilde{Y}_y)$\;
        $(M,s,A,b)\gets $ signed support $\&$ affine\;}

        $c_{M,s}= \max_{i|A_{i,n+1}<0}\left\{\frac{b_i- [A_{i,1},\ldots, A_{i,n}]\cdot \bY^\top}{A_{i,n+1}}\right\}$\;
        $d_{M,s}= \min_{i|A_{i,n+1}>0}\left\{\frac{b_i- [A_{i,1},\ldots, A_{i,n}]\cdot \bY^\top}{A_{i,n+1}}\right\}$\;
        
        $\mathbf{p}\gets \tilde{\bX}((\tilde{\bX}_{M}^{+})_{1:n}\bY-\lambda (\tilde{\bX}_{M}^\top \tilde{\bX}_{M})^{-1}s)-\begin{bmatrix}
    \bY\\ 0\end{bmatrix}$\;
        $\mathbf{q}\gets \tilde{\bX}(\tilde{\bX}_{M}^+)_{n+1}-[\vec{0},1]$\;
        $|(\rs)_y|\gets |\tilde{Y}_y-\hat{\beta}_y(\tilde{\bX})|$\;
    }
    \Else{
    \tcc{Least square fit}
    % $\hat{\beta}_y =\tilde{X}_{M}^+\tilde{Y}-\lambda (\tilde{X}_M^\top \tilde{X}_{M})^{-1}s$\;
    $|(\rs)_y|\gets |\mathbf{p}-\mathbf{q}y|$\;
    }
    }
    $\Ypred = \Big\{y : \text{Rank$(|((\rs)_y)_{n+1}|)$}>\lceil(n+1)(1-\alpha)\rceil\Big\}$\;
\end{algorithm}
